# Supplementary material for: Theoretical Investigation of Performance-Improved Ferroelectric Tunnel Junction Based on Trap-Assisted Tunneling
Source: arXiv:2508.12879 source file (2026-01-03)
Supplement: Supplementary file 1 [file article_SM.tex]

\documentclass[aip,reprint,apl,numerical]{revtex4-1}
\linespread{1.1}
\makeatletter\if@twocolumn\PassOptionsToPackage{switch}{lineno}\else\fi\makeatother

\usepackage{tabulary,graphicx,amsfonts,amsmath,amssymb,amsbsy,bm}
\usepackage[T1]{fontenc}
\usepackage{ragged2e}
\usepackage{bigints}

%%%%%%%%%%%%%%%%%%%%%%%%%%%%%%%%%%%%%%%%%%%%%%%%%%%%%%%%%%%%%%%%%%%%%%%%%%
% Following additional macros are required to function some 
% functions which are not available in the class used.
%%%%%%%%%%%%%%%%%%%%%%%%%%%%%%%%%%%%%%%%%%%%%%%%%%%%%%%%%%%%%%%%%%%%%%%%%%
\usepackage{url,multirow,morefloats,floatflt,cancel,tfrupee}
\makeatletter

\AtBeginDocument{\@ifpackageloaded{textcomp}{}{\usepackage{textcomp}}}
\makeatother
\usepackage{colortbl}
\usepackage{xcolor}
\usepackage{pifont}
\usepackage[nointegrals]{wasysym}
\urlstyle{rm}
\makeatletter

%%%For Table column width calculation.
\def\mcWidth#1{\csname TY@F#1\endcsname+\tabcolsep}

%%Hacking center and right align for table
\def\cAlignHack{\rightskip\@flushglue\leftskip\@flushglue\parindent\z@\parfillskip\z@skip}
\def\rAlignHack{\rightskip\z@skip\leftskip\@flushglue \parindent\z@\parfillskip\z@skip}

%Etal definition in references
\@ifundefined{etal}{}{}

%\if@twocolumn\usepackage{dblfloatfix}\fi
\usepackage{ifxetex}
\ifxetex\else\if@twocolumn\@ifpackageloaded{stfloats}{}{\usepackage{dblfloatfix}}\fi\fi

\AtBeginDocument{
\expandafter\ifx\csname eqalign\endcsname\relax
\def\eqalign#1{\null\vcenter{\def\\{\cr}\openup\jot\m@th
  \ialign{\strut$\displaystyle{##}$\hfil&$\displaystyle{{}##}$\hfil
      \crcr#1\crcr}}\,}
\fi
}

%For fixing hardfail when unicode letters appear inside table with endfloat
\AtBeginDocument{%
  \@ifpackageloaded{endfloat}%
   {\renewcommand\efloat@iwrite[1]{\immediate\expandafter\protected@write\csname efloat@post#1\endcsname{}}}{\newif\ifefloat@tables}%
}%

\def\BreakURLText#1{\@tfor\brk@tempa:=#1\do{\brk@tempa\hskip0pt}}
\let\lt=<
\let\gt=>
\def\processVert{\ifmmode|\else\textbar\fi}

\@ifundefined{subparagraph}{
\def\subparagraph{\@startsection{paragraph}{5}{2\parindent}{0ex plus 0.1ex minus 0.1ex}%
{0ex}{\normalfont\small\itshape}}%
}{}

% These are now gobbled, so won't appear in the PDF.
\newcommand\role[1]{\unskip}
\newcommand\aucollab[1]{\unskip}
  
\@ifundefined{tsGraphicsScaleX}{\gdef\tsGraphicsScaleX{1}}{}
\@ifundefined{tsGraphicsScaleY}{\gdef\tsGraphicsScaleY{.9}}{}
% To automatically resize figures to fit inside the text area
\def\checkGraphicsWidth{\ifdim\Gin@nat@width>\linewidth
	\tsGraphicsScaleX\linewidth\else\Gin@nat@width\fi}

\def\checkGraphicsHeight{\ifdim\Gin@nat@height>.9\textheight
	\tsGraphicsScaleY\textheight\else\Gin@nat@height\fi}

\def\fixFloatSize#1{}%\@ifundefined{processdelayedfloats}{\setbox0=\hbox{\includegraphics{#1}}\ifnum\wd0<\columnwidth\relax\renewenvironment{figure*}{\begin{figure}}{\end{figure}}\fi}{}}
\let\ts@includegraphics\includegraphics

\def\inlinegraphic[#1]#2{{\edef\@tempa{#1}\edef\baseline@shift{\ifx\@tempa\@empty0\else#1\fi}\edef\tempZ{\the\numexpr(\numexpr(\baseline@shift*\f@size/100))}\protect\raisebox{\tempZ pt}{\ts@includegraphics{#2}}}}

\AtBeginDocument{\def\includegraphics{\@ifnextchar[{\ts@includegraphics}{\ts@includegraphics[width=\checkGraphicsWidth,height=\checkGraphicsHeight,keepaspectratio]}}}

\DeclareMathAlphabet{\mathpzc}{OT1}{pzc}{m}{it}

\def\URL#1#2{\@ifundefined{href}{#2}{\href{#1}{#2}}}

%%For url break
\def\UrlOrds{\do\*\do\-\do\~\do\'\do\"\do\-}%
\g@addto@macro{\UrlBreaks}{\UrlOrds}

\edef\fntEncoding{\f@encoding}

\makeatother

\newif\ifmultipleabstract\multipleabstractfalse%
%

%%%%%%%%%%%%%%%%%%%%%%%%%%%%%%%%%%%%%%%%%%%%%%%%%%%%%%%%%%%%%%%%%%%%%%%%%

%%%%%%%%%%%%%%%%%%%%%%%%%%%%%%%%%%%%%%%%%%%%%%%%%%%%%%%%
\usepackage{caption,subcaption,booktabs,fancyhdr,placeins}

%\pagestyle{fancy}
%\fancyhf{}
%\fancyhead[R]{\thepage}
%\renewcommand{\headrulewidth}{0pt}
%\thispagestyle{empty} % 第一页不显示页码
%%%%%%%%%%%%%%%%%%%%%%%%%%%%%%%%%%%%%%%%%%%%%%%%%%%%%%%%

%%% :改成. Figure, Table, Equation, Citation 編號加S
\makeatletter

% 改成[SX] 樣式，編號加S
 % This line requires natbib

 % This line requires natbib

% 改成(SX) 樣式，編號加S

% 改成 Table SX. / Figure SX. 樣式，去掉自動冒號並編號加S
\renewcommand{\fnum@table}{Table~S\arabic{table}.}
\renewcommand{\fnum@figure}{Figure~S\arabic{figure}.}

% 重新定義 caption 格式，不再自動加冒號
\long\def\@makecaption#1#2{%
  \vskip\abovecaptionskip
  \sbox\@tempboxa{#1\ #2}%
  \ifdim \wd\@tempboxa >\hsize
    #1\ #2\par
  \else
    \global \@minipagefalse
    \hb@xt@\hsize{\box\@tempboxa\hfil}%
  \fi
  \vskip\belowcaptionskip}%
\makeatother
%%%

\usepackage{float,newfloat}

\begin{document}

\def\authorCount{2}
\def\affCount{2}

\def\journalTitle{Applied Physics Letters}

\title{\centering \large Supplementary Material\\
Theoretical Investigation of Performance-Improved Ferroelectric Tunnel Junction Based on Trap-Assisted Tunneling }

\author{SHI-XI Kong}
\email{281611631kong@gmail.com}
\affiliation{Department of Electronics and Electrical Engineering\unskip, National Yang Ming Chiao Tung University\unskip, 30010\unskip, Hsinchu\unskip, Taiwan, Republic of China}
\author{Tuo-Hung Hou}
\email{thhou@nycu.edu.tw}
\affiliation{Department of Electronics and Electrical Engineering\unskip, National Yang Ming Chiao Tung University\unskip, 30010\unskip, Hsinchu\unskip, Taiwan, Republic of China}
\affiliation{Institute of Electronics\unskip, National Yang Ming Chiao Tung University\unskip, Hsinchu\unskip, 30010\unskip, Taiwan, Republic of China}

\maketitle \onecolumngrid \vspace{-2em} \hspace{5.9cm}{\Large\textbf{S1. Simulation Method}}

\vspace{1em}

Figure~S1 schematically illustrates the Ni/Al$_2$O$_3$/HZO/BIL/TiN MIFIM-FTJ structure.
The simulated stack follows the experimental configuration reported by Chu \textit{et al.}~\cite{Chu2021TSA}, in which a bottom interfacial layer (BIL) is observed at the HZO/TiN interface in transmission electron microscopy images. Previous studies have attributed this BIL to either monoclinic-phase HZO~\cite{m-phaseBIL} or TiN$_x$O$_y$ formation~\cite{TiNxOyBIL}. In this work, it is modeled as monoclinic-phase HZO.

The ferroelectric (FE) switching, trap dynamics, and electric potential in the MIFIM-FTJ are calculated through an iterative self-consistent scheme. 
The up/down major $P$–$V$ loop of the FE layer is described by the Preisach model~\cite{S1} as
\begin{equation}
F_{u/d}(V) = P_s \tanh[s(V \mp E_c T_{\mathrm{FE}})],
\end{equation}
where the slope factor $s$ is defined as
\begin{equation}
s = \ln \left( \frac{P_s + P_r}{P_s - P_r} \right) / \big( 2 E_c T_{\mathrm{FE}} \big),
\end{equation}
and $P_s$, $P_r$, and $E_c$ denote the saturation polarization, remanent polarization, and coercive field, respectively, while $T_{\mathrm{FE}}$ is the FE layer thickness. 
The thickness dependence of these parameters follows empirical relations obtained from literature~\cite{S2,S3},
\begin{equation}
P_s = k_s T_{\mathrm{FE}}, \quad P_r = k_r T_{\mathrm{FE}}, \quad E_c = k_c T_{\mathrm{FE}}^{-0.61},
\end{equation}
where $k_s$, $k_r$, and $k_c$ are the proportional coefficients.

The minor-loop behavior is modeled by tracking the evolution of the two previous history turning points 
\((V_s, V_n, P_{FE}(V_n))\) and \((V_f, V_p, P_{FE}(V_p))\).~\cite{S4}
A turning point is defined as the instant when the applied voltage across the FTJ reverses its sweep direction. 
\(V_s\) and \(V_f\) denote the smaller and larger applied voltages across the MIFIM-FTJ stack, respectively, while \(V_n\) and \(V_p\) represent the corresponding voltages across the FE layer.
The minor P--V loop is calculated by a linear mapping of the major P--V loop \(F(V)\) as~\cite{S4}
\begin{equation}
P_{\mathrm{FE,u/d}}(V) = m_{u/d}F(V) + c_{u/d},
\end{equation}
where
\begin{equation}
m_{u/d} = \frac{P_{\mathrm{FE,u/d}}(V_n)-P_{\mathrm{FE,u/d}}(V_p)}{F_{u/d}(V_n)-F_{u/d}(V_p)}, \qquad
c_{u/d} = \frac{P_{\mathrm{FE,u/d}}(V_n)F_{u/d}(V_p)-P_{\mathrm{FE,u/d}}(V_p)F_{u/d}(V_n)}{F_{u/d}(V_p)-F_{u/d}(V_n)}.
\end{equation}
The sweep voltage is set from $-\infty \!\rightarrow\! V_f \!\rightarrow\! V_s \!\rightarrow\! V_f \!\rightarrow\! V_s \!\cdots$, initializing the negative saturation state and reproducing the repeated PUND cycles used in experiments. Using Eqs.~(S4)--(S6), the first minor loop \(P_{1,u/d}(V)\) is obtained from the pairs \((-\infty, -\infty, -P_s)\) and \((V_f,V_p,F_u(V_f))\). The subsequent minor loops \(P_{FE}(V)\) converge to an identical trajectory, which can be reconstructed from \((V_f,V_p,F_u(V_f))\) and \((V_s,V_n,P_{1,d}(V_s))\), and are used for the self-consistent calculations.

The trap dynamics are evaluated based on the framework proposed by Guan \textit{et al.}~\cite{S5}, which describes a phonon-assisted inelastic trap-assisted tunneling (TAT) mechanism in HfO$_2$. In a quasi-steady state, the current continuity equation is in the form of
\begin{equation}
(1-f_n)\!\left(R_n^{iT}+R_n^{iB}\right)
-f_n\!\left(R_n^{oT}+R_n^{oB}\right)
+\sum_{m\neq n}\!\!\left[(1-f_n)R_{mn}f_m-f_n R_{nm}(1-f_m)\right]=0,
\end{equation}
where $f_n\in[0,1]$ is the electron occupation probability, $R_{mn}$ is the hopping rate from trap $m$ to $n$, $R^{oT(B)}_n$ denotes the electron hopping rate from trap $n$ to the top (bottom) electrode, and $R^{iT(B)}_n$ represents the hopping rate from the top (bottom) electrode to trap $n$.

The hopping rates between a trap and electrodes are expressed as
\begin{equation}
R_n^{i\,T(B)} \;=\; R_{\mathrm{tunnel}}\,N_{T(B)}\!\left(E_n^{+}\right)\,F^{T(B)}_{\mathrm{in}}\!\left(E_n^{+}\right)\,T^{T(B),+}_n,
\qquad
R_n^{o\,T(B)} \;=\; R_{\mathrm{tunnel}}\,N_{T(B)}\!\left(E_n^{\bullet}\right)\,F^{T(B)}_{\mathrm{out}}\!\left(E_n^{\bullet}\right)\,T^{T(B),\bullet}_n,
\end{equation}
where $R_{\mathrm{tunnel}}$ is the coupling strength between the trap and the electrode, $N_{T(B)}$ denotes the number of states in the top (bottom) electrode at the energy, and $E_n^{+}$ ($E_n^{\bullet}$) is the energy of an empty (filled) trap. $T^{T(B),+}_n$ is the transmission probability from the top (bottom) electrode into the trap, and $T^{T(B),\bullet}_n$ is the transmission probability from the trap into the top (bottom) electrode. They can be calculated using the Wentzel–Kramers–Brillouin (WKB) approximation~\cite{S7} as
\begin{align}
T^{T,+(\bullet)}_n
&= \exp\!\bigg[-2 \int_{0}^{x_{n}} \sqrt{\frac{2m^\ast}{\hbar^2}\,
\max\Big[E_C(x) - E_{n}^{+(\bullet)},0\Big]}\,dx \bigg], \\[2mm]
T^{B,+(\bullet)}_n
&= \exp\!\bigg[-2 \int_{x_{n}}^{T_{total}} \sqrt{\frac{2m^\ast}{\hbar^2}\,
\max\Big[E_C(x) - E_{n}^{+(\bullet)},0\Big]}\,dx \bigg],
\end{align}
where $E_c$ is the conduction band energy, $m^\ast$ is the effective electron mass, $x_{n}$ is the distance of trap n from the top electrode, and $T_{total}$ are the total thickness of the FTJ, respectively.
$F_{\mathrm{in/out}}^{T(B)}$ denote the Fermi integrals giving the number of filled/empty states in the top (bottom) electrode that can exchange electrons with trap~$n$, defined as
\begin{align}
F_{\mathrm{in}}^{T(B)}(E_n^+)
  &= \bigintss_{E_{n}^+}^{+\infty}
     \vcenter{\hbox{$\dfrac{dE}{1+\exp\!\left[\dfrac{E - E_F^{T(B)}}{kT}\right]}$}}, \\[4pt]
F_{\mathrm{out}}^{T(B)}(E_n^{\bullet})
  &= \bigintss_{-\infty}^{E_{n}^{\bullet}}
     \vcenter{\hbox{$\dfrac{dE}{1+\exp\!\left[\dfrac{E_F^{T(B)} - E}{kT}\right]}$}}.
\end{align}
Here $E_F^{T(B)}$ is the Fermi level of the electrodes.

The hopping rate between two traps is expressed as
\begin{equation}
R_{mn} = R_0 \exp\!\left[-\frac{r_{nm}}{a_0} + \frac{\max[E_m^{\bullet} - E_n^{+},0]}{kT}\right],
\end{equation}
by the Mott hopping model~\cite{ambegaokar1971hopping, kopperberg2021consistent},
where $R_0$ is the vibration frequency of an electron in a trap, 
$r_{nm}=|x_m-x_n|$ is the distance between the two traps,
and $a_0$ is the attenuation length of the electron wave function.

The self-consistent calculation is performed through two iterative loops, 
where the outer loop iterates the FE switching 
and the inner loop iterates the trap dynamics and potential.
Initially, in the outer loop, the voltage across the FE layer, $V_{\mathrm{FE}}$, is guessed under a particular applied voltage. 
Subsequently, an initial electron occupation probability $f_n^{\mathrm{ini}}$ is assumed in the inner loop.
The electric potential $V(x)$ is then calculated by solving the 1D Poisson equation
\begin{equation}
\frac{d^2V(x)}{dx^2}
= -\frac{1}{\kappa(x)\varepsilon_0}\Big[\rho_{\mathrm{FE}}(x) + \rho_{\mathrm{trap}}(x)\Big].
\end{equation}
where $\kappa$ is the dielectric constant and $\varepsilon_0$ is the vacuum permittivity.
The FE bound charge is represented by
\begin{equation}
\rho_{\mathrm{FE}}(x)
= P_{\mathrm{FE}}\,[\delta(x-(T_{\mathrm{TIL}}+T_{\mathrm{FE}}))-\delta(x-T_{\mathrm{TIL}})],
\end{equation}
and the charge of trap is given by
\begin{equation}
\rho_{\mathrm{trap}}=\sum_n\rho_{\mathrm{trap},n} = -\sum_n\frac{q}{A}\,(f_n-f_n^0)\delta(x-x_n),
\end{equation}
where A is the cross-sectional area of FTJ, and $f_n^0$ = 1 or 0 for donor-like and acceptor-like traps, respectively.  
Although traps may have different charge states, they can be effectively modeled as a superposition of donor- and acceptor-type states without loss of generality.
From the obtained electric potential $V(x)$, the conduction band profile $E_C(x)$ can be calculated accordingly. 
The occupation $f_n$ is then updated through Eqs.~(S6)–(S12).
This iteration continues until the occupation variation $\Delta f_n = |f_n^{\mathrm{out}} - f_n^{\mathrm{ini}}|$ converges below a predefined tolerance $\epsilon_1$.  
The converged potential is then fed back to the outer loop to update $V_{\mathrm{FE}}$, following the same convergence condition $\Delta V_{\mathrm{FE}}\le\epsilon_2$, ensuring a self-consistent solution.
The applied voltages at the turning points are first self-consistently obtained to construct the minor P--V loop from Eqs.~(S1)–(S5), after which the remaining bias points are calculated accordingly.

Based on previous self-consistent calculations, the total current density is then calculated by direct tunneling (DT), Fowler–Nordheim (FN) tunneling, and trap-assisted tunneling (TAT) mechanisms. 
Fowler–Nordheim tunneling is similar to direct tunneling, representing the same quantum-tunneling phenomenon.
The direct/Fowler–Nordheim tunneling current density is calculated by the Tsu–Esaki model~\cite{tsu1973tunneling} as
\begin{equation}
J_{\mathrm{DT/FN}} = \frac{4\pi m^\ast q}{h^3}
\int_{E_{\min}}^{E_{\max}} T(E)\, \mathcal{N}(E)\, dE,
\end{equation}
where \(E_{\min}\) is the higher conduction-band edge of the two electrodes and \(E_{\max}\) is the conduction-band edge of the dielectric. 
The transmission probability is given by the WKB approximation as~\cite{S7}
\begin{equation}
T(E) = \exp\!\left[
-\frac{2}{\hbar}
\int_{0}^{T_{\mathrm{total}}}
\sqrt{2m^\ast\,\max\big(E_c(x)-E,0\big)}\, dx
\right],
\end{equation}
and the supply function from the two electrodes is
\begin{equation}
\mathcal{N}(E) = k_B T
\ln\!\left(
\frac{1+\exp\!\big[\frac{E - E_F^{T}}{k_B T}\big]}
     {1+\exp\!\big[\frac{E - E_F^{B}}{k_B T}\big]}
\right).
\end{equation}
And the TAT current is obtained from the net electron transfer between traps and top (or bottom) electrodes as
\begin{equation}
J_{\mathrm{TAT}} = -\frac{q}{A} \sum_{n}\Big[(1 - f_n) R_n^{i\,T} - f_n R_n^{o\,T}\Big]=\frac{q}{A} \sum_{n}\Big[(1 - f_n) R_n^{i\,B} - f_n R_n^{o\,B}\Big].
\end{equation}
The total current is therefore determined by the sum of direct/Fowler–Nordheim and trap-assisted tunneling contributions, i.e.,
\begin{equation}
J_{\mathrm{total}} = J_{\mathrm{DT/FN}} + J_{\mathrm{TAT}}.
\end{equation}

In this work, the electron affinities $\chi$ are set to 1.58~eV and 2.2~eV for Al$_2$O$_3$~\cite{Al2O3EA} and HZO~\cite{HZOEA}, respectively. 
The work function $\phi$ of Ni is 5.15~eV~\cite{NiWF}, while TiN exhibits a reported range of 4.1--5.3~eV~\cite{TiNWF}. For simplicity, a representative value of 5.15~eV is adopted. 
The dielectric constants $\kappa$ are 9 for Al$_2$O$_3$~\cite{Al2O3DEconstant} and 30/22 for the ferroelectric orthorhombic and non-ferroelectric monoclinic phases of HZO~\cite{HZOophaseDEconstant,HZOmphaseDEconstant}, corresponding to the FE layer and the BIL, respectively. 
The trap-related and tunneling parameters follow Guan \textit{et al.}~\cite{S5}, where the vibration frequency of an electron in a trap is $R_0 = 10^{12}\,\mathrm{Hz}$, 
the attenuation length of the electron wave function is $a_0 = 0.33\,\mathrm{nm}$, 
the electronic coupling factor between the electrode and the dielectric layer is $R_{\mathrm{tunnel}}^0 N^{T(B)} = 10^{14}\,\mathrm{Hz}$, and the effective electron mass is $m^\ast = 0.1m_0$, where $m_0$ is the free electron mass. The temperature is fixed at $300~\mathrm{K}$.
The trap sites are assumed to be located at the Al$_2$O$_3$/HZO interface for simplicity in modeling, where interfacial defects are expected to preferentially form during film deposition at the heterogeneous interface. 
The empty and filled trap energy levels are assumed to be split by a constant $\Delta E=0.1\ eV$ around a central trap level $E_T$ distributed in 1.1–2.9~eV below the conduction band of the FE layer, i.e.,
\begin{equation}
2.9\ eV>\lim_{\delta x \to 0^+}[E_{c}(T_{\mathrm{TIL}}+\delta x)-E_{T,n}]=E_{c,\mathrm{FE}}(T_{\mathrm{TIL}})-E_{T,n}>1.1\ eV,
\end{equation}
\begin{equation}
E_n^{+} = E_{\mathrm{T},n} + \frac{\Delta E}{2},\  E_n^{\bullet} = E_{\mathrm{T},n} - \frac{\Delta E}{2},
\end{equation}
following the range reported for HfO$_2$~\cite{HfO2trapenergyrange}, which lies energetically closer to the Fermi level than that of Al$_2$O$_3$ (1.7–2.0~eV below the conduction band of the TIL)~\cite{Al2O3trapenergyrange}. 
For simplicity, the traps are assumed to be uniformly distributed within the energy range, and a charge-neutrality level (CNL) is introduced, above which the traps behave as acceptor-like and below which they act as donor-like states. The CNL is set in the middle of the energy range. Its exact value is not critical, as it only shifts the pinning level without altering the overall pinning behavior discussed in Fig.3.
To quantify the interfacial trap population, a trap surface density $N_T$ is defined as the total number of traps normalized by the device cross-sectional area, i.e., $N_T = ($number of traps$)/A$. The associated trap charge density $Q_T$ is then expressed as $Q_T = \sum_n -q\,(f_n - f_n^0)/A$. Accordingly, in the self-consistent calculation, the iterative update of individual $f_n$ in the inner loop can be equivalently represented by the convergence of $Q_T$, which simplifies the self-consistent calculation.

The major $P$–$V$ loop and the trap surface density $N_T$ were determined by fitting the experimental data.
Table~S1 summarizes the extracted fitting parameters and the layer thicknesses of the 1.5-nm Al$_2$O$_3$/3-nm HZO/0.6-nm BIL and the 3-nm HZO/0.6-nm BIL FTJs.

\begingroup
\makeatletter
\long\def\@makecaption#1#2{%
  \vskip\abovecaptionskip
  #1\ #2\par
  \vskip\belowcaptionskip}%
\makeatother
\begin{figure*}[!htbp]
\centering
\makeatletter\IfFileExists{images/FigureS3.png}{\includegraphics[width=0.4\textwidth]{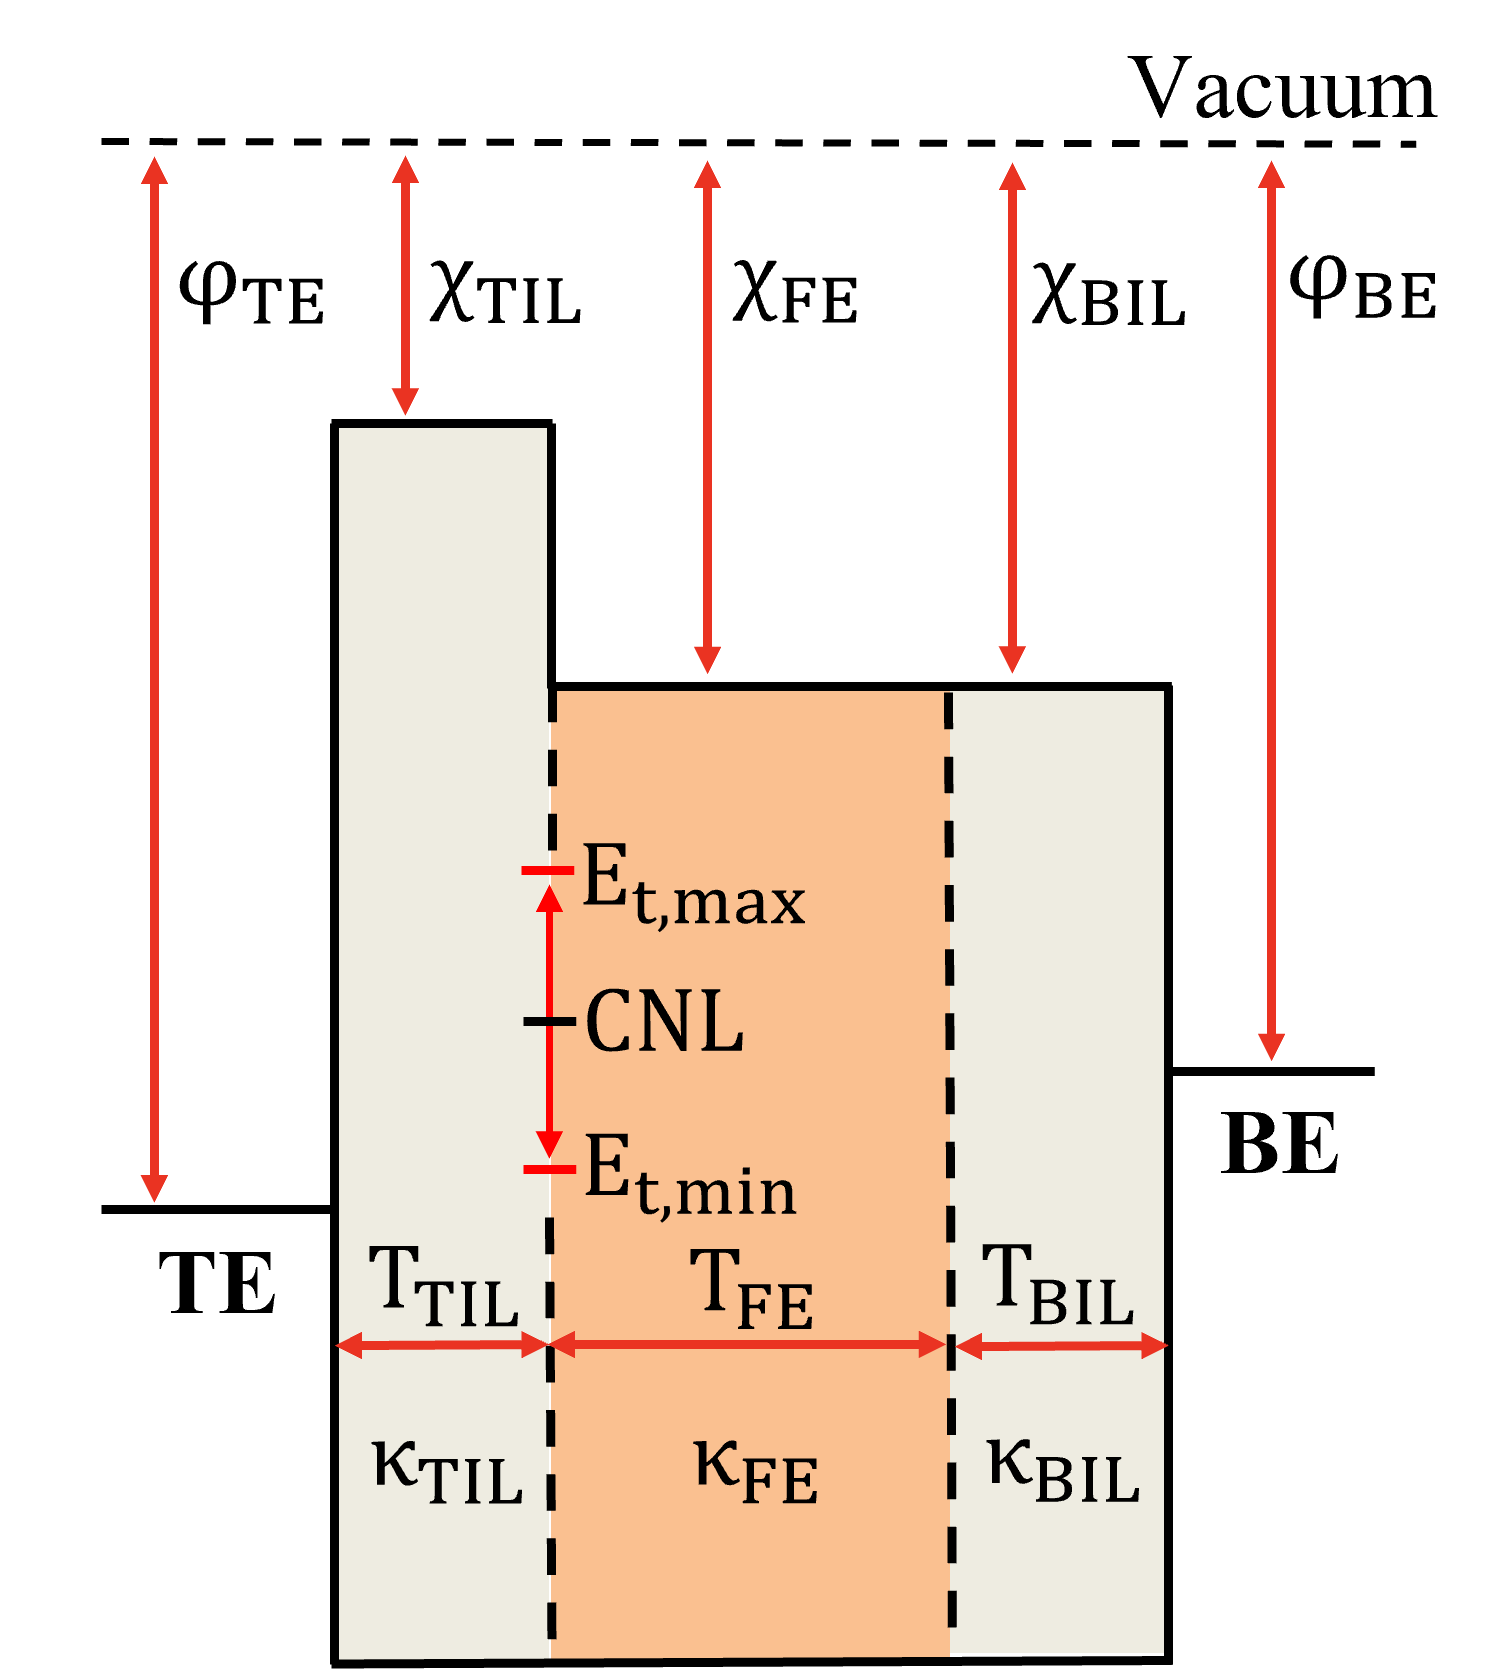}}{\includegraphics[width=0.4\textwidth]{FigureS1.png}}
\makeatother 
\caption{\raggedright The schematic of the device structure and trap conditions of the simulated FTJ.}
\label{FigureS1}
\end{figure*}
\endgroup

\begingroup
\makeatletter
\long\def\@makecaption#1#2{%
  \vskip\abovecaptionskip
  #1\ #2\par
  \vskip\belowcaptionskip}%
\makeatother
\begin{table}[!h]
\caption{\raggedright The extracted fitting parameters and the layer thicknesses of the 1.5-nm Al\textsubscript{2}O\textsubscript{3}/3-nm HZO/0.6-nm BIL and the 3-nm HZO/0.6-nm BIL FTJ.}
\centering
\renewcommand{\arraystretch}{1.5} % 行高调整
\setlength{\tabcolsep}{10pt} % 列间距调整
\begin{tabular}{@{} >{\raggedright\arraybackslash}m{3cm} >{\raggedright\arraybackslash}m{5cm} >{\raggedright\arraybackslash}m{3cm} >{\raggedright\arraybackslash}m{3cm} @{}}
\toprule
Symbol          & Quantity                      & w/ 1.5nm Al\textsubscript{2}O\textsubscript{3} & w/o 1.5nm Al\textsubscript{2}O\textsubscript{3} \\ 
\midrule
$k_s(= P_s/T_\mathrm{FE})$      & Saturation Polarization Coefficient    & $3\;\mu\mathrm{C}/\mathrm{cm}^2 \cdot \mathrm{nm}$ & $3\;\mu\mathrm{C}/\mathrm{cm}^2 \cdot \mathrm{nm}$     \\
$k_r(= P_r/T_\mathrm{FE})$      & Remnant Polarization Coefficient       & $2.997\;\mu\mathrm{C}/\mathrm{cm}^2 \cdot \mathrm{nm}$ & $2.997\;\mu\mathrm{C}/\mathrm{cm}^2 \cdot \mathrm{nm}$     \\
$k_c(= E_c/T_\mathrm{FE}^{0.61})$ & Coercive Field Coefficient            & $2.5\;\mathrm{MV}/\mathrm{cm} \cdot \mathrm{nm}^{-0.61}$ & $2.5\;\mathrm{MV}/\mathrm{cm} \cdot \mathrm{nm}^{-0.61}$ \\
$N_\mathrm{T}$           & Trap Surface Density                  & $10^{12}\;\mathrm{cm}^{-2}$              & $0\;\mathrm{cm}^{-2}$ \\
$T_\mathrm{TIL}$                & TIL Thickness                         & $1.5\;\mathrm{nm}$                          & $0\;\mathrm{nm}$ \\
$T_\mathrm{FE}$                 & FE Thickness                          & $3\;\mathrm{nm}$                            & $3\;\mathrm{nm}$  \\
$T_\mathrm{BIL}$                & BIL Thickness                         & $0.6\;\mathrm{nm}$                          & $0.6\;\mathrm{nm}$ \\
\bottomrule
\end{tabular}
\label{table:values}
\end{table}
\endgroup

\maketitle
\clearpage
\centering {\Large\textbf{S2. Thickness scaling of conventional FTJ}}

\vspace{1em}

\justifying
As shown in Fig.~S2, the \ensuremath{T_{\mathrm{total}}} dependence of the conventional FTJ exhibits a similar trend to that of the TAT-based FTJ. However, at \ensuremath{T_{\mathrm{total}} = 3.1~\mathrm{nm}}, the conventional FTJ shows a significantly lower performance, with a \ensuremath{J_{\mathrm{ON}}} below \ensuremath{1~\mathrm{A/cm^2}} and an $J_{\mathrm{ON}}/J_{\mathrm{OFF}}$ ratio less than 1.1---both substantially inferior to those of the TAT-based FTJ.

\bgroup
\fixFloatSize{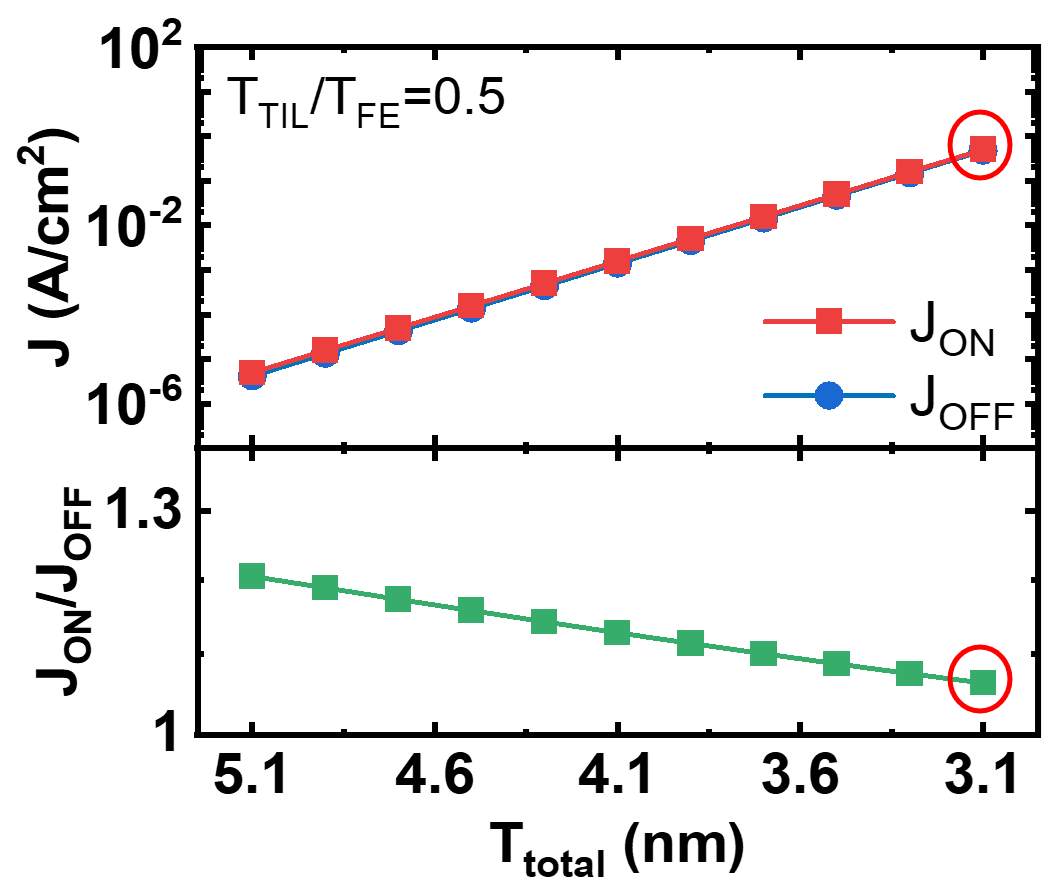}
\begin{figure*}[!htbp]
\centering \makeatletter\IfFileExists{images/FigureS2.png}{\includegraphics{images/FigureS2.png}}{\includegraphics{FigureS2.png}}
\makeatother 
\caption{\raggedright{Thickness scaling of conventional FTJ under \ensuremath{V_{\mathrm{write}}=1\ \mathrm{V}} and \ensuremath{V_{\mathrm{read}}=0.1\ \mathrm{V}}.}}
\label{FigureS2}
\end{figure*}
\egroup

\centering {\Large\textbf{S3. Trap Condition Refinement After Device Structure Optimization}}

\vspace{1em}

\justifying
With the optimal device structure condition of the TAT-based FTJ, further refinement of trap conditions is conducted. Figure~S3(a) and S3(b) present the optimization of \ensuremath{E_{\mathrm{T}}} and \ensuremath{N_{\mathrm{T}}}, respectively.

\bgroup
\fixFloatSize{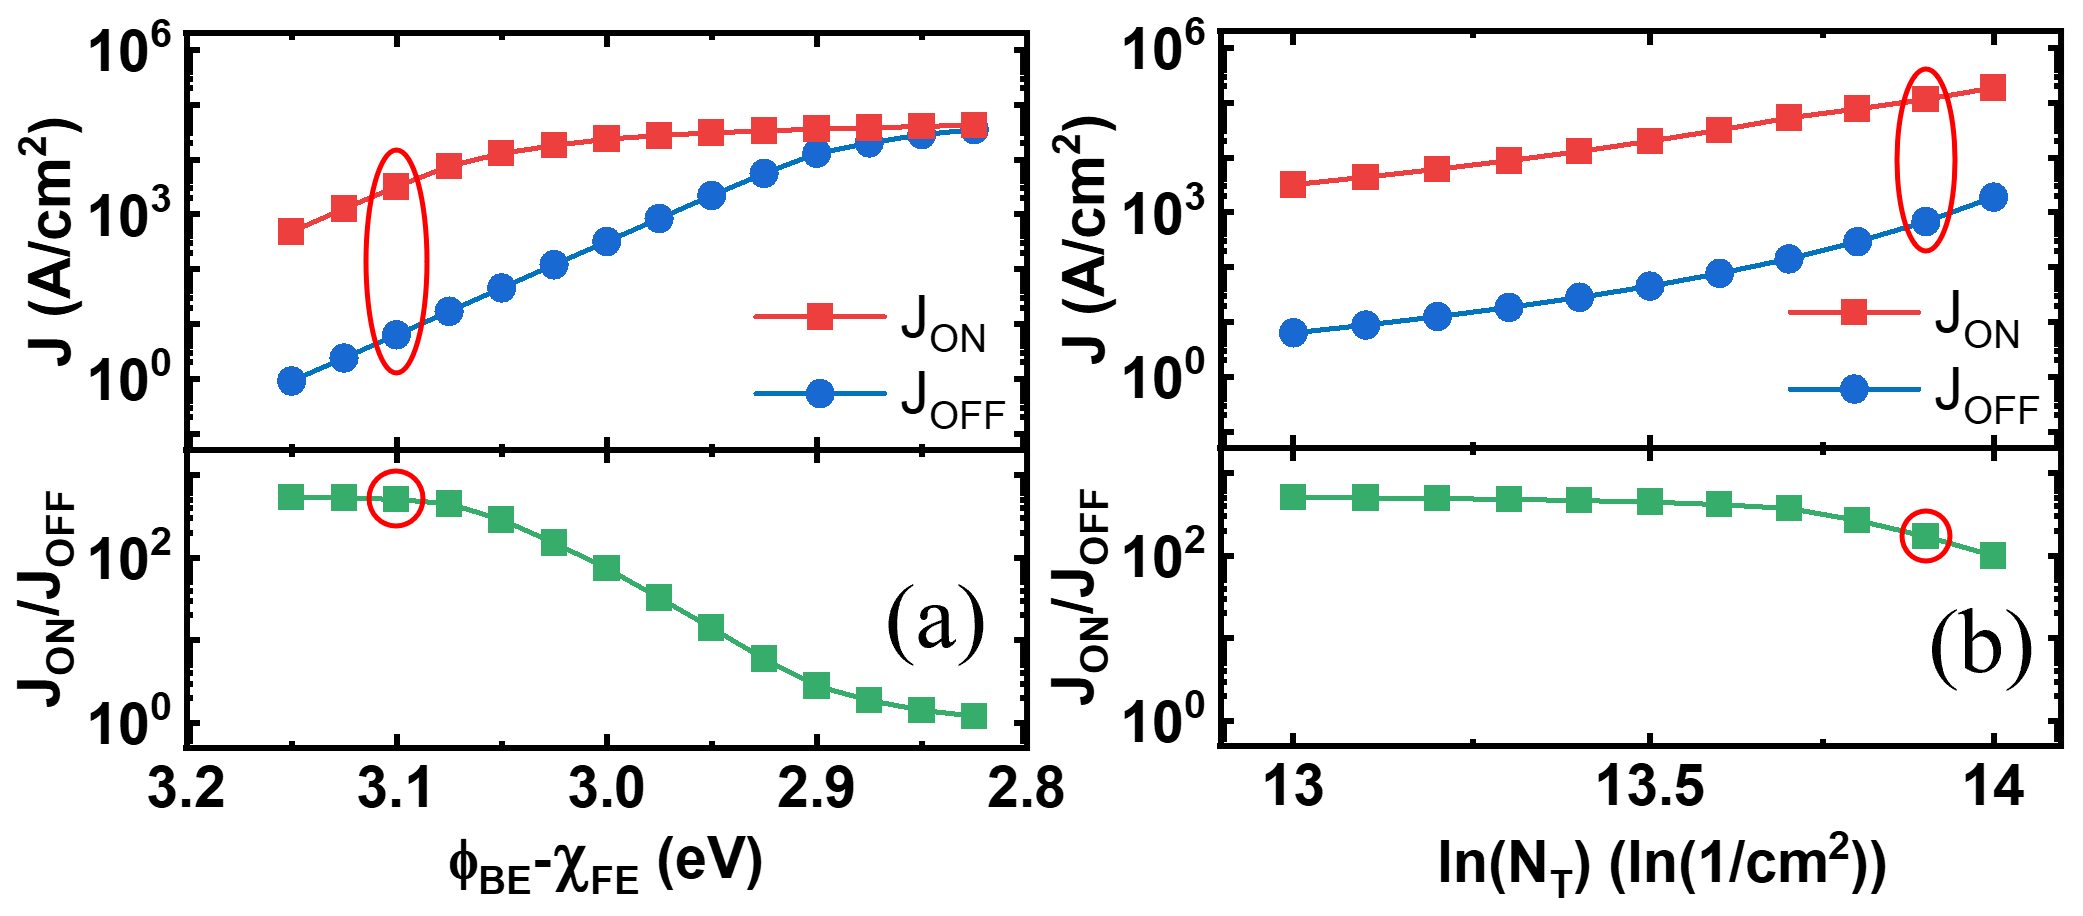}
\begin{figure*}[!htbp]
\centering \makeatletter\IfFileExists{images/FigureS3.png}{\includegraphics{images/FigureS3.png}}{\includegraphics{FigureS3.png}}
\makeatother 
\caption{\raggedright{(a) Continuum-level \ensuremath{E_{\mathrm{T}}} and (b) \ensuremath{N_{\mathrm{T}}} dependence of \ensuremath{J_{\mathrm{TAT}}} of the 0.35-nm Al\ensuremath{_{2}}O\ensuremath{_{3}}/2.15-nm HZO/0.6-nm BIL TAT-based FTJ under \ensuremath{V_{\mathrm{write}}=1\ \mathrm{V}} and \ensuremath{V_{\mathrm{read}}=0.1\ \mathrm{V}}.}}
\label{FigureS3}
\end{figure*}
\egroup

\bibliography{article_SM}
\end{document}
